# Supplementary material for: BlendGAN: Learning and Blending the Internal Distributions of Single Images by Spatial Image-Identity Conditioning
Source: arXiv:2212.01589 source file (2022-12-03)
Supplement: Supplementary file 1 [file sm.tex]

\section{Supporting Image Manipulation Applications}
Similarly to SinGAN~\cite{shaham2019singan}, our model can be used for tasks like image editing and paint-to-image. Figure~\ref{fig:multi_editing} shows several examples of those tasks. Note, however, that in contrast to SinGAN, our model is trained once on all images (four in this case), and can be used at inference time on each one of them separately.

\begin{figure*}[t]
\centering
\includegraphics[width=0.6\linewidth]{figures/multi/editing-painting_v2.pdf}
\caption{\textbf{Performing image manipulation tasks on several images.} Our model is trained on four images and at inference time can perform different tasks on each of them individually.}
\label{fig:multi_editing}
\end{figure*}

\section{Evaluating the cropping mechanism}
To evaluate our cropping mechanism, we compare the performance of our method to SinGAN and ConSinGAN (both with their default configurations). This is summarized in \cref{tab:cropping}. 
We tested our method with a cropping window size of $128\times 128$, and a batch size of $2$. We measure the average per-pixel diversity \cite{shaham2019singan}, SIFID \cite{shaham2019singan} and the NIQE \cite{niqe} scores over $50$ random samples generated from each of the $50$ images of the SinGAN user study dataset. As can be seen, the cropping training scheme performs similarly to that of the vanilla SinGAN and ConSinGAN, although the generator sees only a portion of the training image in each optimization step. Importantly, this particular scheme allows faster training through parallel computing, as well as handling of higher resolution images.

\begin{table}[h]
\small
\begin{center}
\begin{tabular}{c c c c}
Method & Diversity & SIFID & NIQE\\ \hline \hline 
SinGAN & $0.22 \pm 0.14$ & $0.15 \pm 0.07$ & $7.34 \pm 3.43$ \\
ConSinGAN & $0.24 \pm 0.17$ & $0.15 \pm 0.08$ & $7.43 \pm 3.51$ \\
Ours & $0.21 \pm 0.15$ & $0.15 \pm 0.06$ & $7.33 \pm 3.29$ \\
\end{tabular}
\end{center}
\caption{\textbf{Vanilla vs.~Cropping}. Diversity, SIFID and NIQE scores. Our cropping training scheme performs similarly to that of the vanilla SinGAN, even though in each optimization step the generator only sees a portion of the image.
}
\label{tab:cropping}
\end{table}

\section{Training on large images}
The cropping mechanism allows us to train on significantly larger images than what is usually possible with single-image-GAN models, for a given memory consumption budget. As an example, Fig.~\ref{fig:pantheon} shows generation results for a $400\times660$ image, which is larger than the maximal size that can be handled by \cite{shaham2019singan,gur2020hierarchical,hinz2021improved,sushko2021one} on the same hardware (an $11$Gb-RAM GPU). Figure \ref{fig:gordon} shows an additional example of generation results for a $400\times600$ image.

\input{figures/pantheon/pantheon}
\input{figures/gordon/gordon}

\section{Memory consumption.}
\Cref{fig:memory} shows the memory consumption of the vanilla SinGAN training method and of our cropping scheme, when training on a single image. The original scheme experiences a steep increase in memory consumption as a function of the size of the training image, and becomes impractical already for moderately sized images. With cropping, on the other hand, memory consumption grows moderately. This allows training on larger images using the same hardware.

\begin{figure}[h]
\centering
\includegraphics[width=.65\linewidth]{./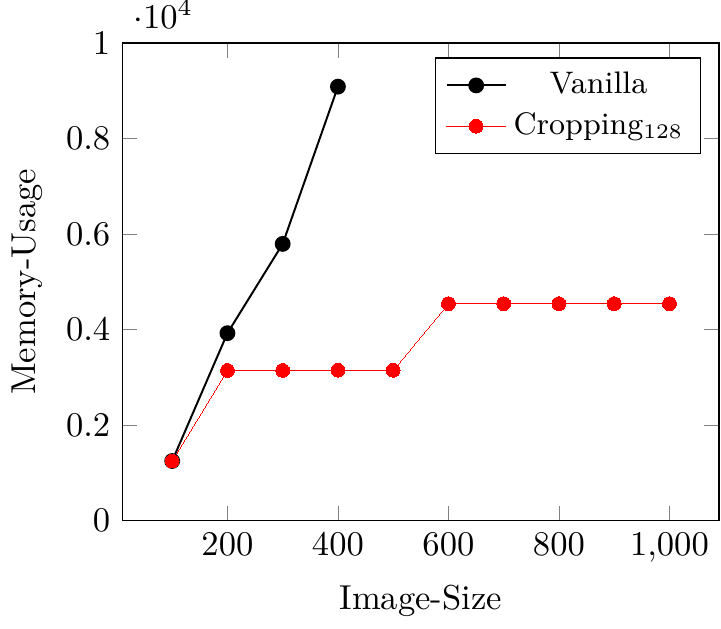}
\caption{\textbf{Memory usage.} We compare the vanilla SinGAN training method to our cropping scheme in terms of memory training usage. Training on large images is possible with our method due to its bounded memory consumption.}
\label{fig:memory}
\end{figure}

\section{Optimization}
The optimization process of BlendGAN is identical to that of the original SinGAN~\cite{shaham2019singan}, with one important difference: instead of using a single image in each gradient step, we perform  optimization on batches. For scales corresponding to image sizes smaller than the crop size (where we use the full images), the batch size is set to be the number of images. For scales where the image is larger than the crop, we use a batch size of twice the number of images. In both cases, we ensure that all image identities appear in each gradient step. 

\section{Architectural Details}
Tables~\ref{tab:arch_generator} and~\ref{tab:arch_discriminator} provide descriptions of the network architectures we use for all the experiments. We use leaky ReLU with slope $0.2$. At the coarsest scale, we use $32$ channels per block, and every four scales the number of channels per block increases by a factor of two. We use convolutions with no padding. 

\begin{table*}
    \begin{center}
		\begin{tabular}{c c}
			Generator & sBasicBlock\\  
			\begin{tabular}{ c }
				\hline \hline
				$z_i, (\widetilde{x}_{i+1})\uparrow^r, \text{img}_{\text{id}}  \in \mathbb{R}^{h\times w \times 3}$\\
				$z_i + (\widetilde{x}_{i+1})\uparrow^r$\\
				Conv., $3\times 3$, $C_{i}$\\
				sBasicBlock, $C_{i}$\\
				sBasicBlock, $C_{i}$\\
				sBasicBlock, $C_{i}$\\
				Conv., $3\times 3$, $3$\\
				$+(\widetilde{x}_{i+1})\uparrow^r$\\ 
				Tanh\\ \\
			\end{tabular} &  
			\begin{tabular}{ c } 
				\hline \hline
				\includegraphics[width=0.35\columnwidth]{figures/schemes/sbasicblock.pdf}
			\end{tabular}
		\end{tabular}
		\caption{\textbf{Generator architecture.} The number of channels is set to be $C_{i} = \min\{512, 32 \cdot 2^{\lfloor i / 4 \rfloor}\}$. As opposed to \cite{park2019semantic}, here all of SPADE's convolutions are $1\times 1$.}
		\label{tab:arch_generator}
	\end{center}
\end{table*}

\begin{table*}
    \begin{center}
		\begin{tabular}{c c}
			Discriminator & BasicBlock\\  
			\begin{tabular}{ c }
				\hline \hline
				$x_i  \in \mathbb{R}^{h\times w \times 3}$\\ \\
				Conv., $3\times 3$, $C_{i}$\\
				BasicBlock, $C_{i}$\\
				BasicBlock, $C_{i}$\\
				BasicBlock, $C_{i}$\\
				Conv., $3\times 3$, $1$\\ \\ \\ \\
			\end{tabular} &  
			\begin{tabular}{ c } 
				\hline \hline
				\includegraphics[width=0.35\columnwidth]{figures/schemes/basicblock.pdf}
			\end{tabular}
		\end{tabular}
		\caption{\textbf{Discriminator architecture.} The number of channels is set to be $C_{i} = \min\{512, 32 \cdot 2^{\lfloor i / 4 \rfloor}\}$.}
		\label{tab:arch_discriminator}
	\end{center}
\end{table*}

\section{Additional Results}
We now provide several additional qualitative results for BlendGAN, as in Sec.~4 of the main text (please see many more examples in the supplementary video). Specifically, we have the following:
\begin{enumerate}
\item Figure~\ref{fig:clip_sm} shows additional morphing results after training with semantic loss.
\item Figure~\ref{fig:sampling_with_map_sm} shows  additional examples of our model's capability to accommodate spatially varying non-categorical identity structures at inference time, allowing each pixel to be sampled from one of the training image identities.
\item Additional illustrations of our model's ability to spatially blend natural images are provided in Figures ~\ref{fig:sm_spatial} and \ref{fig:sampling_with_map_3images}. Particularly, here we show various spatial transition patterns between random samples generated by our model.
\item Additional demonstration of our model's ability to interpolate between two images while maintaining photo-realism is shown in Figure~\ref{fig:image_morphing}. Figure~\ref{fig:sample_morphing} illustrates morphing between random samples, rather than between the images themselves. Figure~\ref{fig:morphing_3images} shows morphing between three images. 
\item In Fig.~\ref{fig:consingan} we demonstrate the incorporation of our framework into ConSinGAN~\cite{hinz2021improved}.
\end{enumerate}

\input{figures/clip/clip-sm.tex}
\input{figures/sampling-with-map/sampling-with-map-sm.tex}

\input{figures/blending/blending-sm}

\input{figures/blending/blending-3images-sm.tex}

\input{figures/morphing/morphing-fixed-sm}
\input{figures/morphing/morphing-sampled-sm}

\input{figures/morphing/fruit1-fruit2-fruit5-mat.tex}
\input{figures/morphing/morphing-fixed-3-images.tex}

\input{figures/consingan/consingan.tex}
